# Supplementary material for: Efficient Parallel Output-Sensitive Edit Distance
Source: arXiv:2306.17461 source file (2023-08-31)
Supplement: Supplementary file 1 [file appendix-hashtable.tex]

\section{Illustration of Building and Query for \hashtab{}}
\label{app:hashillustration}
\cref{fig:hash-illustration} show the contruction and query of the \hashtab{}.
\input{figures/hash.tex}

% For the \fname{Compare} call in \cref{algo:hashtab} we know that if the start point of the string 
% is also the start of any block, we can directly get the value from the \hashtab{}. 
% Otherwise there are three parts we need to combine(\cref{fig:hash-query-ill}). 
% For example, assume there we call the \fname{Compare}(5, 21, 1) on the finished \hashtab{(A)} and \hashtab{(B)}, 
% which aims to compare the hash value of two substrings $A[5..16]$ and $B[10..21]$ with both length
%  $2^1 * t = 12$, where $t$ is the size of the blocks. The hash value query for both $A$ and $B$ are 
%  under the same procedure. We can combine the three parts by hashcombine operation ($\hashcombine$), which 
%  includes the suffix of the uncomplete part at the beginning ($A[5] * p^2 + A[6] * p + A[7]$ for $A$), the \hashtab{} value including $2^1$ blocks,
%   and the prefix value of the uncomplete part up to the end point ($B[20] * p + B[21]$ for $B$). 

The construction keeps the values of two parts:
\begin{enumerate}
    \item[1)] The \hashtab{} $T$, which stores the hash value of substrings in corresponding block ranges. For example, in the \cref{fig:hash-illustration}(a)
    $T[0][x_2]$ and $T[0][x_3]$ will keep the hash values of the two blocks starting from $A[x_2]$ and $A[x_3]$, respectively.
    For the substrings contain both the blue and yellow blocks, we calculate the value and write it to $T[1][x_2]$
    \item[2)] Prefix and suffix values of all the element in the entire string. The $\prefixhash{A}[x_1]$ shown in \cref{fig:hash-illustration}(a) keeps the
    prefix value from start of the same block up to $A[x_1]$, while $\suffixhash{A}[x_1]$ takes the hashcombined value from $A[x_1]$ up to the end of the same block.
\end{enumerate}

\cref{fig:hash-illustration}(b) is an example for the value retrieving while applying \fname{Compare} function. We can see
from the figure that the value within query range consists three pieces: 1) the prefix hash value $\prefixhash{B}[x_s]$, 2) the block-range
hash value $T[0][x_B]$ in the \hashtab{}, 3) and the suffix value $\suffixhash{B}[x_d]$. We combine the three parts as the hash value
of the substring slice from $B[x_s]$ to $B[x_d]$.
